# Supplementary material for: NavigateDiff: Visual Predictors are Zero-Shot Navigation Assistants
Source: arXiv:2502.13894 source file (2025-02-19)
Supplement: Supplementary file 1 [file 6_appendix.tex]

\section*{APPENDIX}

Appendixes should appear before the acknowledgment.
